# Supplementary material for: Electronic excitations and spin interactions in chromium trihalides from embedded many-body wavefunctions
Source: arXiv:2208.02195 ancillary file (2022-08-03)
Supplement: Supplementary file 1 [file SupportingInformation.pdf]

Supporting Information

**Electronic excitations and spin interactions in  
chromium trihalides from embedded  
many-body wavefunctions**

Ravi Yadav,<sup>†,‡</sup> Lei Xu,<sup>¶</sup> Michele Pizzochero,<sup>§</sup> . . . ,<sup>†</sup> and Oleg V. Yazyev<sup>\*,†,‡</sup>

<sup>†</sup>*Institute of Physics, Ecole Polytechnique Fédérale de Lausanne (EPFL),  
1015 Lausanne, Switzerland*

<sup>‡</sup>*National Centre for Computational Design and Discovery of Novel Materials (MARVEL),  
Ecole Polytechnique Fédérale de Lausanne (EPFL), 1015 Lausanne, Switzerland*

<sup>¶</sup>*Theoretical Division, Los Alamos National Laboratory,  
Los Alamos, NM 87545, United States*

<sup>§</sup>*School of Engineering and Applied Sciences, Harvard University,  
Cambridge, MA 02138, United States*

E-mail: oleg.yazyev@epfl.ch

## Supporting Note S1: One-site quantum chemistry calculations

Multiplet structures (Table I in the main text) and intra-site magnetic interactions (Table II in the main text) are obtained using the finite-size model shown in Figure 1(b) in the main text. This model consists of a central unit that comprises a single  $\text{CrX}_6$  ( $X=\text{Cl}, \text{I}$ ) octahedron treated with many-body wavefunctions, surrounded by the three nearest-neighbor octahedra. These latter octahedra account for the finite charge distribution in the vicinity of the central unit and are treated at the Hartree-Fock level. The remaining crystalline environment is modeled by arrays of point charges reproducing the ionic Madelung potential in the cluster region.<sup>1</sup> All-electron basis functions of quadruple-zeta quality supplemented with  $f$ -polarization functions are used for the  $\text{Cr}^{3+}$  ion in the reference unit.<sup>2</sup> The  $\text{Cr}^{3+}$  ions centered in the three nearest-neighbor octahedra are described as closed-shell  $\text{Sc}^{3+}$  ions with an all-electron basis set of triple-zeta quality.<sup>2</sup> For Cl ligands in  $\text{CrCl}_3$ , an all-electron basis set of triple-zeta quality is employed.<sup>3</sup> The Cl atoms in the octahedra surrounding the reference unit are represented with an all-electron basis sets of double-zeta quality.<sup>3</sup> In the case of  $\text{CrI}_3$ , energy-consistent relativistic pseudopotentials along with quadruple-zeta quality basis sets for the valence shells of I atoms in the reference octahedron,<sup>4</sup> while energy-consistent relativistic pseudopotentials along with triple-zeta quality basis sets are used for the I atoms in the nearest-neighbor octahedra.<sup>4</sup>

CASSCF wavefunctions are variationally optimized for an average of low-lying seven quartet and five doublet states. In the subsequent MRCI calculations, we account for dynamic correlation effects by including single- and double-excitations involving the  $t_{2g}$  orbitals of the  $\text{Cr}^{3+}$  ions and the  $p$  valence shells of halogen ligands within the central unit.<sup>5</sup> Calculations are performed using the MOLPRO package.<sup>6</sup>

## Supporting Note S2: Quantum chemistry simulation of XAS and RIXS spectra

The simulation of XAS and RIXS spectra (Figure 2 in the main text) is carried out at the CASSCF level using the finite-size model shown in Supporting Figure S1(a).<sup>7</sup> This model consists of a single  $\text{CrX}_6$  ( $X = \text{Cl, I}$ ) octahedron surrounded by an array of point charges to reproduce the ionic Madelung potential of the crystalline environment.<sup>1</sup> For the  $\text{Cr}^{3+}$  ion, we use an all-electron triple-zeta Douglas-Kroll basis sets with diffuse functions, along with weighted core-valence sets aug-cc-pwCVTZ-DK<sup>2</sup> to describe core-valence correlation effects. For the halogen ligands, we employ an all-electron triple-zeta Douglas-Kroll basis sets with diffuse functions aug-cc-pVTZ-DK.<sup>3</sup> To compute the  $\text{Cr}^{3+} 3d^3$  valence-excited states at the CASSCF level, we consider an active space comprising five  $3d$  orbitals ( $t_{2g}$  and  $e_g$ ) and three electrons. Ten spin-triplet and forty spin-doublet valence states associated with this manifold are obtained in the state-averaged complete active space self-consistent field optimization. The Pipek-Mezey localization scheme,<sup>8</sup> as implemented in Ref. 6, is adopted for localizing the orbitals of the halogen atoms. All these valence-excited states enter the spin-orbit coupling calculations at the CASSCF level. Spin-orbit coupling (SOC) effects are accounted for by diagonalizing the Breit-Pauli spin-orbit matrix in the basis of the scalar relativistic (SR) states.<sup>9</sup> Calculations are performed with the MOLPRO package.<sup>6</sup> The source code is modified and compiled in order to compute up to 800 SR states in the CASSCF module, thus allowing these states to be coupled in the subsequent SOC calculations. The resulting  $d$  excitation energies up to 4 eV are listed in Supporting Tables S2 and S3.

For the determination of the  $2p^5 3d^4$  core-hole states, which are the final states in the  $L$ -edge X-ray absorption process and the intermediate states in the  $L$ -edge RIXS process, the active space is defined in terms of nine electrons and five Cr  $3d$  orbitals, in addition to three Cr  $2p$  orbitals, these latter being frozen to an occupation restriction that allows a maximum of five electrons. The self-consistent field optimization is performed for an average of 15 spin sextet, 150 spin quartet and 285 spin doublet states associated with the  $2p^5 3d^4$  configurations. All these states further enter the SOC calculations, leading to a total of 1260

spin-orbit-coupled states.

The dipole transition matrix elements between wavefunctions expressed in terms of the nonorthogonal orbitals for the  $3d^3$  and  $2p^5 3d^4$  groups of states are derived according to the procedure described in Ref. 10. The XAS and RIXS scattering geometry and the directions of polarization are adjusted according to the setup of experimental measurements described in Ref. 11, also shown in Supporting Figure S1(b). Linearly polarized X-rays are incident at an angle  $\theta$  with the plane of the sample, this latter being oriented in such a way that the  $c$ -axis points to the surface normal. The scattering angle,  $\alpha$ , between the incoming and outgoing light beams is set to  $40^\circ$  and the incident angle,  $\theta$ , to  $50^\circ$ . The incoming light is linearly polarized, either perpendicularly to the scattering plane ( $\sigma$  polarization) or within the scattering plane ( $\pi$  polarization). For the outgoing radiation, we carry out a summation over the two independent polarization directions.

For the analysis of the *ab initio* wavefunctions, we rely on a local coordinate frame  $\{x, y, z\}$  with the  $x$ ,  $y$  and  $z$  components pointing along  $a$ ,  $b$  and  $c$  axes of the  $\text{CrCl}_3/\text{CrI}_3$  unit cell, respectively. The rotation of the  $\sigma$ ,  $\pi$  and  $\pi'$  (introduced as outgoing  $\pi$  polarization) vectors as function of the angle  $\theta$  is described by the following geometrical relations

$$\begin{aligned}\vec{D}_\sigma &= \vec{D}_y, \\ \vec{D}_\pi &= \vec{D}_x \sin \theta + \vec{D}_z \cos \theta, \\ \vec{D}_{\pi'} &= \vec{D}_x \sin(\theta + \alpha) + \vec{D}_z \cos(\theta + \alpha),\end{aligned}\tag{1}$$

where  $\vec{D}_\epsilon^{kl} = \langle \Psi_{\text{fs}}^k | \vec{\epsilon} \cdot \vec{R} | \Psi_{c^*}^l \rangle \langle \Psi_{\text{fs}}^k | \vec{\epsilon} \cdot \vec{R} | \Psi_{c^*}^l \rangle$  is the dipole transition matrix elements. The expression of the X-ray absorption cross section<sup>12,13</sup> involves the summation over the ground state and core-excited states

$$\begin{aligned}I^{\text{XAS}}(\hbar\omega, \epsilon, \theta) &= 4\pi^2\alpha \sum_j \frac{1}{g_{\text{gs}}} \sum_l \hbar\omega \left| \langle \Psi_{c^*}^l | \vec{D}_\epsilon | \Psi_{\text{gs}}^j \rangle \langle \Psi_{c^*}^l | \vec{D}_\epsilon | \Psi_{\text{gs}}^j \rangle \right|^2 \\ &\times \frac{\Gamma_{c^*}/2\pi}{(E_{\text{gs}}^j + \hbar\omega - E_{c^*}^l)^2 + (\Gamma_{c^*})^2/4}.\end{aligned}\tag{2}$$

The RIXS double differential cross-section is obtained by summing over the outgoing polarization directions<sup>12,14</sup>

$$\begin{aligned}
I^{RIXS}(\hbar\omega, \hbar\omega', \epsilon, \theta) &= \frac{d^2\sigma_{\vec{k}, \epsilon}^{RIXS}}{d\Omega' d\hbar\omega'} = \\
&\frac{\alpha^2 \hbar^2}{e^4 c^2} \omega \omega'^3 \sum_{\epsilon'} \sum_j \frac{1}{g_{gs}} \sum_k \left| \sum_l \frac{\langle \Psi_{fs}^k | \vec{D}_{\epsilon'} | \Psi_{c^*}^l \rangle \langle \Psi_{fs}^k | \vec{D}_{\epsilon'} | \Psi_{c^*}^l \rangle \langle \Psi_{c^*}^l | \vec{D}_{\epsilon} | \Psi_{gs}^j \rangle \langle \Psi_{c^*}^l | \vec{D}_{\epsilon} | \Psi_{gs}^j \rangle}{E_{gs}^j + \hbar\omega - E_{c^*}^l + (i\Gamma_{c^*}/2)} \right|^2 \\
&\times \frac{\Gamma_{fs}/2\pi}{(E_{gs}^j + \hbar\omega - E_{fs}^k - \hbar\omega')^2 + (\Gamma_{fs})^2/4}. \tag{3}
\end{aligned}$$

In Equations 2 and 3,  $\alpha$  is the fine structure constant,  $\hbar\omega$  is the energy of the incoming photons,  $\hbar\omega'$  is the energy of outgoing photons, while  $\epsilon$  and  $\epsilon'$  are polarizations of the incoming and outgoing photons, respectively. For  $I^{XAS}$ , the summations take into account all core-hole (intermediate) states and the possible degeneracy of the ground state  $g_{gs}$ . For  $I^{RIXS}$ , the summations take into account all core-hole  $2p^5 3d^4$  (intermediate) states and  $2p^6 3d^3$  (final) states and the possible degeneracy of the ground state,  $g_{gs}$ . The lifetimes of the core-excited and valence-excited states are  $\Gamma_{c^*}$  and  $\Gamma_{fs}$ , respectively. The natural widths  $\Gamma_{c^*}$  are set to 0.4 eV for both  $\text{CrCl}_3$  and  $\text{CrI}_3$ . The natural widths  $\Gamma_{fs}$  are set to 0.3 eV for  $\text{CrCl}_3$  and 0.35 eV for  $\text{CrI}_3$ , that is, the same values adopted in the reference experimental work of Ref. 11. The RIXS spectra of  $\pi$ -polarization direction are directly compared to the corresponding experimental spectra.<sup>11</sup>

### Supporting Note S3: Two-site quantum chemistry calculations

Inter-site magnetic interactions (Table III in the main text) are obtained using the finite-size model shown in Figure 1(c) in the main text. This model consists of a central unit that comprises two edge-sharing  $\text{Cr}_2\text{X}_{10}$  ( $X = \text{Cl}, \text{Br}, \text{I}$ ) octahedra treated with many-body wavefunctions, surrounded by the four nearest-neighbor octahedra. These latter octahedra account for the finite charge distribution in the vicinity of the central unit and are treated at the Hartree-Fock level. The remaining crystalline environment is modeled by arrays of point charges reproducing the ionic Madelung potential in the cluster region.<sup>1</sup> All-electron basis functions of quadruple-zeta quality were used for the  $\text{Cr}^{3+}$  ions<sup>2</sup> in the two-octahedra central unit. The bridging halogen ligands are modeled with an all-electron quintuple-zeta quality basis set,<sup>3,15</sup> while, for the bridging I ligand, energy-consistent relativistic pseudopotentials along with quintuple-zeta quality basis sets for the valence shells are employed.<sup>4</sup> The remaining ligand atoms in the central region are described using a triple-zeta quality basis set in the case of Cl and Br atoms,<sup>3,15</sup> and energy-consistent relativistic pseudopotentials along with triple-zeta quality basis sets in the case of I atoms.<sup>4</sup>  $\text{Cr}^{3+}$  ions centered at the octahedra adjacent to the reference unit are described as closed-shell  $\text{Sc}^{3+}$  ions and an all-electron triple-zeta basis functions.<sup>2</sup> The ligands belonging to these octahedra are modeled with double-zeta quality basis set for the Cl and Br atoms<sup>3,15</sup> and energy-consistent relativistic pseudopotentials along with double-zeta quality basis sets for the I atoms.<sup>4</sup>

CASSCF wavefunctions are variationally optimized for an average of one septet, quintet, triplet and singlet states, which are mainly of  $t_{2g}^3 - t_{2g}^3$  character. In addition to  $t_{2g}^3 - t_{2g}^3$  direct exchange between the nearest-neighbor sites, these wavefunctions consist of a finite-weight contribution that stems from inter-site excitations of  $t_{2g}^4 - t_{2g}^2$  type.<sup>5</sup> MRCI calculations account for single- and double-excitations involving the  $t_{2g}$  orbitals of the  $\text{Cr}^{3+}$  ions and the  $p$  valence shells of the bridging halogen ligands. In the treatment of spin-orbit effects, one septet, quintet, triplet and singlet states are considered, both in CASSCF and MRCI approaches. Calculations are performed using the MOLPRO package.<sup>6</sup>

**Supporting Table S1: Effect of in-plane compressive and tensile lattice strain ( $\epsilon$ ) on the multiplet structure of  $\text{CrCl}_3$ , as obtained at the MRCI level of theory, using the finite-size model shown in Figure 1(b) in the main text. Energies are given in eV and referenced to the ground state.**

|                            | $\epsilon = -2\%$ | $\epsilon = 0\%$ | $\epsilon = +2\%$ |
|----------------------------|-------------------|------------------|-------------------|
| ${}^4A_2 (t_{2g}^3 e_g^0)$ | 0.00              | 0.00             | 0.00              |
| ${}^4T_2 (t_{2g}^2 e_g^1)$ | 1.79, 1.79, 1.85  | 1.67, 1.68, 1.70 | 1.38, 1.45, 1.50  |
| ${}^2E (t_{2g}^3 e_g^0)$   | 2.39, 2.40        | 2.21, 2.21       | 2.36, 2.37        |
| ${}^4T_2 (t_{2g}^2 e_g^1)$ | 2.78, 2.80, 2.84  | 2.50, 2.52, 2.59 | 2.25, 2.35, 2.41  |
| ${}^2T_1 (t_{2g}^3 e_g^0)$ | 2.49, 2.51, 2.52  | 2.31, 2.33, 2.34 | 2.48, 2.49, 2.51  |
| ${}^2T_1 (t_{2g}^2 e_g^1)$ | 3.35, 3.36, 3.38  | 3.03, 3.05, 3.07 | 3.23, 3.26, 3.28  |
| ${}^2A_1 (t_{2g}^2 e_g^1)$ | 3.72              | 3.47             | 3.42              |
| ${}^2T_1 (t_{2g}^2 e_g^1)$ | 3.99, 4.01, 4.04  | 3.76, 3.77, 3.78 | 3.67, 3.70, 3.75  |
| ${}^4T_1 (t_{2g}^1 e_g^2)$ | 4.43, 4.44, 4.48  | 4.05, 4.07, 4.08 | 3.88, 3.93, 3.97  |

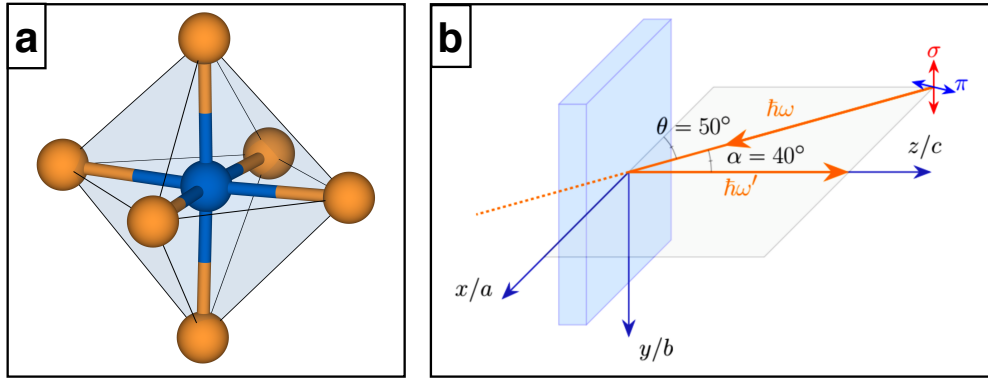

**Supporting Figure S1:** (a) Finite-size model used in the simulation of the XAS and RIXS spectra. Blue and orange spheres represent chromium and halogen atoms, respectively. The model is embedded in an array of points charges (not shown) to ensure charge neutrality and reproduce the crystalline environment. (b) RIXS scattering geometry used in our *ab initio* calculations, analogous to the experimental setup adopted in Ref. 11.

**Supporting Table S2: Relative energies (eV) at the CASSCF and CASSCF+SOC level of theory for the  $\text{Cr}^{3+} 3d^3$  multiplet structure in  $\text{CrCl}_3$ , as obtained using the finite-size model shown in Supporting Figure S1(a). Each CASSCF+SOC value denotes a spin-orbit doublet. For the  $^4T$  and  $^2T$  states, only the lowest and highest components are given.**

|                         | Relative energy (eV) |               |
|-------------------------|----------------------|---------------|
|                         | CASSCF               | CASSCF+SOC    |
| $^4A_2(t_{2g}^3)$       | 0.00                 | 0.00          |
| $^4T_2(t_{2g}^2 e_g^1)$ | 1.62; 1.66; 1.66     | 1.61 ... 1.67 |
| $^2E(t_{2g}^3)$         | 2.27; 2.27           | 2.27; 2.28    |
| $^2T_1(t_{2g}^3)$       | 2.36; 2.41; 2.41     | 2.36 ... 2.42 |
| $^4T_2(t_{2g}^2 e_g^1)$ | 2.56; 2.56; 2.67     | 2.55 ... 2.67 |
| $^2T_2(t_{2g}^3)$       | 3.19; 3.19; 3.29     | 3.18 ... 3.30 |
| $^2A(t_{2g}^2 e_g^1)$   | 3.53                 | 3.54          |
| $^2T_1(t_{2g}^2 e_g^1)$ | 3.75; 3.83; 3.83     | 3.75 ... 3.84 |
| $^2T_2(t_{2g}^2 e_g^1)$ | 3.95; 3.95; 4.01     | 3.93 ... 4.00 |

**Supporting Table S3: Relative energies (eV) at the CASSCF and CASSCF+SOC level of theory for the  $\text{Cr}^{3+} 3d^3$  multiplet structure in  $\text{CrI}_3$ , as obtained using the finite-size model shown in Supporting Figure S1(a). Each CASSCF+SOC value denotes a spin-orbit doublet. For the  ${}^4T$  and  ${}^2T$  states, only the lowest and highest components are given.**

|                          | Relative energy (eV) |               |
|--------------------------|----------------------|---------------|
|                          | CASSCF               | CASSCF+SOC    |
| ${}^4A_2(t_{2g}^3)$      | 0.00                 | 0.00          |
| ${}^4T_2(t_{2g}^2e_g^1)$ | 1.37; 1.41; 1.41     | 1.36 ... 1.41 |
| ${}^2E(t_{2g}^3)$        | 2.19; 2.19           | 2.19; 2.19    |
| ${}^4T_2(t_{2g}^2e_g^1)$ | 2.22; 2.22; 2.29     | 2.22 ... 2.30 |
| ${}^2T_1(t_{2g}^3)$      | 2.29; 2.33; 2.33     | 2.30 ... 2.33 |
| ${}^2T_2(t_{2g}^3)$      | 2.99; 2.99; 3.09     | 2.99 ... 3.09 |
| ${}^2A(t_{2g}^2e_g^1)$   | 3.22                 | 3.22          |
| ${}^2T_1(t_{2g}^2e_g^1)$ | 3.37; 3.45; 3.45     | 3.37 ... 3.45 |
| ${}^2T_2(t_{2g}^2e_g^1)$ | 3.59; 3.59; 3.63     | 3.58 ...      |
| ${}^4T_1(t_{2g}^1e_g^2)$ | 3.59; 3.79; 3.79     | ... 3.79      |
| ${}^2E(t_{2g}^2e_g^1)$   | 3.91; 3.91           | 3.90; 3.92    |

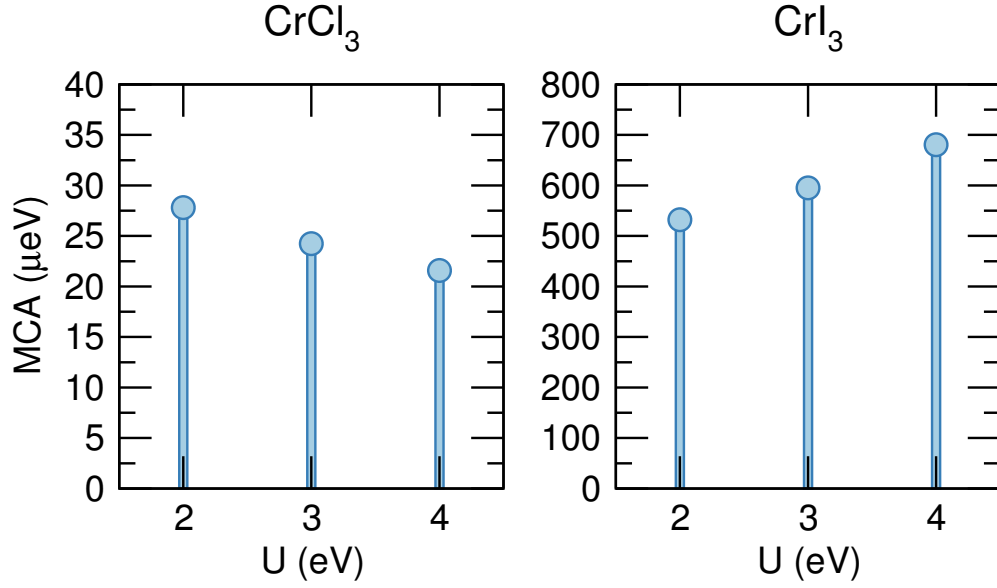

**Supporting Figure S2:** Magnetocrystalline anisotropy energy (MCA) of CrCl<sub>3</sub> (left panel) and CrI<sub>3</sub> (right panel) — as obtained from Hubbard-corrected, periodic density-functional theory calculations<sup>16,17</sup> — for increasing values of on-site repulsion  $U$ . The MCA is found to be larger in CrI<sub>3</sub> than CrCl<sub>3</sub> because of the stronger spin-orbit interactions in the former trihalide than the latter. Contrary to CrI<sub>3</sub>, the experimentally observed in-plane magnetization axis of CrCl<sub>3</sub> originates from the dominant contribution of the shape anisotropy (w.r.t. MAE) to the overall magnetic anisotropy energy, as discussed in Ref. 18. These calculations have been performed with VASP,<sup>19–22</sup> using a cutoff on kinetic energy of 450 eV and a  $k$ -mesh of  $9 \times 6 \times 9$  points.

**Supporting Table S4: Heisenberg exchange interactions in  $\text{CrX}_3$  ( $X = \text{Cr}, \text{Br}, \text{I}$ ) obtained by considering the isotropic bilinear Heisenberg Hamiltonian (i.e., neglecting the biquadratic and inter-site anisotropic terms in Equation 3 of the main text.**

|             | $\text{CrCl}_3$ |       | $\text{CrBr}_3$ |       | $\text{CrI}_3$ |       |
|-------------|-----------------|-------|-----------------|-------|----------------|-------|
|             | CASSCF          | MRCI  | CASSCF          | MRCI  | CASSCF         | MRCI  |
| $J_1$ (meV) | -0.69           | -1.08 | -0.67           | -1.28 | -0.66          | -1.42 |

**Supporting Table S5: Inter-site magnetic interactions in CrBr<sub>3</sub>, i.e., bilinear ( $J_1$ ) and biquadratic ( $J_2$ ) exchange couplings, symmetric anisotropy ( $\Gamma_{xy}$ ,  $\Gamma_{yz}$ ,  $\Gamma_{zx}$ ) and Kitaev ( $K$ ) parameters.**

|                                    | CASSCF                | MRCI                  |
|------------------------------------|-----------------------|-----------------------|
| $J_1$ (meV)                        | -0.61                 | -1.21                 |
| $J_2$ (meV)                        | -0.05                 | -0.05                 |
| $\Gamma_{xy}$ (meV)                | $-6.9 \times 10^{-4}$ | $-0.8 \times 10^{-3}$ |
| $\Gamma_{yz} = -\Gamma_{zx}$ (meV) | $-6.9 \times 10^{-4}$ | $-0.9 \times 10^{-3}$ |
| $K$ (meV)                          | $-8.2 \times 10^{-3}$ | -0.01                 |

## References

- (1) Klintonberg, M.; Derenzo, S.; Weber, M. Accurate crystal fields for embedded cluster calculations. *Computer Physics Communications* **2000**, *131*, 120.
- (2) Balabanov, N. B.; Peterson, K. A. Systematically convergent basis sets for transition metals. I. All-electron correlation consistent basis sets for the 3d elements Sc-Zn. *The Journal of Chemical Physics* **2005**, *123*, 064107.
- (3) Woon, D. E.; Dunning, T. H. Gaussian basis sets for use in correlated molecular calculations. III. The atoms aluminum through argon. *The Journal of Chemical Physics* **1993**, *98*, 1358.
- (4) Peterson, K. A.; Shepler, B. C.; Figgen, D.; Stoll, H. On the spectroscopic and thermochemical properties of ClO, BrO, IO, and their anions. *The Journal of Physical Chemistry A* **2006**, *110*, 13877.
- (5) Helgaker, T.; Jørgensen, P.; Olsen, J. *Molecular Electronic-Structure Theory*; Wiley, Chichester, 2000.
- (6) Werner, H. J.; Knowles, P. J.; Knizia, G.; Manby, F. R.; Schütz, M. Molpro: A general-purpose quantum chemistry program package. *WIREs Computational Molecular Science* **2012**, *2*, 242.
- (7) Xu, L. *Ab initio modeling of the electronic structure of d-metal systems and of resonant inelastic x-ray scattering responses*; Ph.D. thesis, TU Dresden, Germany, 2019.
- (8) Pipek, J.; Mezey, P. G. A fast intrinsic localization procedure applicable for *ab initio* and semiempirical linear combination of atomic orbital wave functions. *The Journal of Chemical Physics* **1989**, *90*, 4916.
- (9) Berning, A.; Schweizer, M.; Werner, H.-J.; Knowles, P. J.; Palmieri, P. Spin-orbit ma-

- trix elements for internally contracted multireference configuration interaction wavefunctions. *Molecular Physics* **2000**, *98*, 1823.
- (10) Mitrushchenkov, A.; Werner, H.-J. Calculation of transition moments between internally contracted MRCI wave functions with non-orthogonal orbitals. *Molecular Physics* **2007**, *105*, 1239.
- (11) Shao, Y. C.; Karki, B.; Huang, W.; Feng, X.; Sumanasekera, G.; Guo, J.-H.; Chuang, Y.-D.; Freelon, B. Spectroscopic Determination of Key Energy Scales for the Base Hamiltonian of Chromium Trihalides. *The Journal of Physical Chemistry Letters* **2021**, *12*, 724.
- (12) van Veenendaal, M. *Theory of Inelastic Scattering and Absorption of X-Rays*; Cambridge: Cambridge University Press, 2015.
- (13) Als-Nielsen, J.; McMorrow, D. *Elements of Modern X-ray Physics*; Wiley, 2011.
- (14) Bogdanov, N. A.; Bisogni, V.; Kraus, R.; Monney, C.; Zhou, K.; Schmitt, T.; Geck, J.; Mitrushchenkov, A. O.; Stoll, H.; van den Brink, J. et al. Orbital breathing effects in the computation of x-ray *d*-ion spectra in solids by *ab initio* wave-function-based methods. *Journal of Physics: Condensed Matter* **2017**, *29*, 035502.
- (15) Wilson, A. K.; Woon, D. E.; Peterson, K. A.; Dunning, T. H. Gaussian basis sets for use in correlated molecular calculations. IX. The atoms gallium through krypton. *The Journal of Chemical Physics* **1999**, *110*, 7667.
- (16) Perdew, J. P.; Burke, K.; Ernzerhof, M. Generalized gradient approximation made simple. *Physical Review Letters* **1996**, *77*, 3865.
- (17) Dudarev, S. L.; Botton, G. A.; Savrasov, S. Y.; Humphreys, C. J.; Sutton, A. P. Electron-energy-loss spectra and the structural stability of nickel oxide: An LSDA+U study. *Physical Review B* **1998**, *57*, 1505.

- (18) Xue, F.; Hou, Y.; Wang, Z.; Wu, R. Two-dimensional ferromagnetic van der Waals  $\text{CrCl}_3$  monolayer with enhanced anisotropy and Curie temperature. *Physical Review B* **2019**, *100*, 224429.
- (19) Kresse, G.; Hafner, J. Ab initio molecular dynamics for liquid metals. *Physical Review B* **1993**, *47*, 558.
- (20) Kresse, G.; Furthmüller, J. Efficient iterative schemes for ab initio total-energy calculations using a plane-wave basis set. *Physical Review B* **1996**, *54*, 11169.
- (21) Kresse, G.; Furthmüller, J. Efficiency of *ab-initio* total energy calculations for metals and semiconductors using a plane-wave basis set. *Computational Materials Science* **1996**, *6*, 15.
- (22) Blöchl, P. E. Projector augmented-wave method. *Physical Review B* **1994**, *50*, 17953.
